# Supplementary material for: The Fragility of Noise Estimation in Kalman Filter: Optimization Can Handle Model-Misspecification
Source: arXiv:2104.02372 source file (2022-06-30)
Supplement: Supplementary file 1 [file supp.tex]

% \documentclass{article}

% % if you need to pass options to natbib, use, e.g.:
% %     \PassOptionsToPackage{numbers, compress}{natbib}
% % before loading neurips_2022

% % ready for submission
% % \usepackage{neurips_2022}

% % to compile a preprint version, e.g., for submission to arXiv, add add the
% % [preprint] option:
%     \usepackage[preprint]{neurips_2022}

% % to compile a camera-ready version, add the [final] option, e.g.:
% %     \usepackage[final]{neurips_2022}

% % to avoid loading the natbib package, add option nonatbib:
% %    \usepackage[nonatbib]{neurips_2022}

% \usepackage[utf8]{inputenc} % allow utf-8 input
% \usepackage[T1]{fontenc}    % use 8-bit T1 fonts
% \usepackage{hyperref}
% \usepackage{url}
% \usepackage{booktabs}       % professional-quality tables
% \usepackage{amsfonts}       % blackboard math symbols
% \usepackage{nicefrac}       % compact symbols for 1/2, etc.
% \usepackage{microtype}      % microtypography
% \usepackage{xcolor}         % colors

% \usepackage{graphicx}
% \usepackage{amsthm}
% \usepackage{amssymb}
% \usepackage{amsmath}
% \usepackage{mathtools}
% \usepackage{dirtytalk}
% \usepackage{floatrow}
% \usepackage{subcaption}
% \usepackage{wrapfig}
% \usepackage[section]{placeins}
% \usepackage[noend,ruled,vlined]{algorithm2e}
% \usepackage{color}
% \usepackage{soul}
% \usepackage{ulem}
% \usepackage{xr}

% \setlength{\textfloatsep}{6pt}

% % Table float box with bottom caption, box width adjusted to content
% \newfloatcommand{capbtabbox}{table}[][\FBwidth]

% \theoremstyle{definition}
% \newtheorem{definition}{Definition}[section]
% \newtheorem{method}{Method}
% \newtheorem{claim}{Claim}[section]
% \newtheorem{lemma}{Lemma}[section]

% \newcommand{\ra}[1]{\hl{#1}}
% % \newcommand{\ra}[1]{#1}
% \newcommand{\rac}[2]{
% 	\hl{#1}
%     {\protect\footnote{\textcolor{red}{#2}}}
% }
% \newcommand{\rdac}[3]{\textcolor{red}{\sout{#1}}\hl{#2}
% 	{\protect\footnote{\textcolor{red}{#3}}}
% }
% \newcommand{\rda}[2]{\textcolor{red}{\sout{#1}}\hl{#2}}
% \newcommand{\rd}[1]{{\textcolor{red}{\sout{{#1}}}}}

% % cross-reference to supplementary material
% \makeatletter
% \newcommand*{\addFileDependency}[1]{% argument=file name and extension
%   \typeout{(#1)}
%   \@addtofilelist{#1}
%   \IfFileExists{#1}{}{\typeout{No file #1.}}
% }
% \makeatother
% \newcommand*{\myexternaldocument}[1]{%
%     \externaldocument{#1}%
%     \addFileDependency{#1.tex}%
%     \addFileDependency{#1.aux}%
% }
% \myexternaldocument{main}

% % \title{Kalman Filter Is All You Need: Optimization Works When Noise Estimation Fails}
% % \title{Rethinking Kalman Filter: Optimization Works When Noise Estimation Fails}
% % \title{Practical Kalman Filter: Optimization Can Handle Model-Misspecification}
% % \title{The Fragility of Noise Estimation in Kalman Filter}
% \title{Supplementary Material}
% % \\ The Fragility of Noise Estimation in Kalman Filter: Optimization Can Handle Model-Misspecification}

% \author{
%   Ido Greenberg \\ %\thanks{Use footnote for providing further information about author (webpage, alternative address)---\emph{not} for acknowledging funding agencies.} \\
%   Technion, Israel \\
%   \texttt{gido@campus.technion.ac.il}
%   \And
%   Shie Mannor \\
%   Technion, Israel \\
%   Nvidia Research
%   \And
%   Netanel Yannay \\
% }

% \begin{document}

% \maketitle


% %%%%%%%%%%%%%%%%%%%%%%%%%%%%%%%%%%%%%%%%%%%%%%%%%
% %%%%%%%%%%%%%%%%%%%%%%%%%%%%%%%%%%%%%%%%%%%%%%%%%

% % \section*{Table of Contents}
% \setcounter{tocdepth}{1}
% \tableofcontents
% \newpage
% \appendix
% \setcounter{figure}{9}
% \setcounter{section}{2}

% %%%%%%%%%%%%%%%%%%%%%%%%%%%%%%%%%%%%%%%%%%%%%%%%%
% %%%%%%%%%%%%%%%%%%%%%%%%%%%%%%%%%%%%%%%%%%%%%%%%%

% \section{Preliminaries: Recurrent Neural Networks}
% \label{sec:preliminaries_extended}

% % \subsection{Recurrent Neural Networks}
% % \label{sec:preliminaries_rnn}

% \textit{Neural networks} (NN) are parametric functions, usually constructed as a sequence of matrix-multiplications with some non-linear differentiable transformation between them. NNs are known to be able to approximate complicated functions, given that the right parameters are chosen. Optimization of the parameters of NNs is a field of vast research for decades, and usually relies on gradient-based methods, that is, calculating the errors of the NN with relation to some training-data of inputs and their desired outputs, deriving the errors with respect to the network's parameters, and moving the parameters against the direction of the gradient.

% \textit{Recurrent neural networks} (RNN)~\citep{RNN} are NN that are intended to be iteratively fed with sequential data samples, and that pass information (the \textit{hidden state}) over iterations. Every iteration, the hidden state is fed to the next copy of the network as part of its input, along with the new data sample.
% \textit{Long Short Term Memory} (LSTM)~\citep{LSTM} is an architecture of RNN that is particularly popular due to the linear flow of the hidden state over iterations, which allows to capture memory for relatively long term.
% The parameters of a RNN are usually optimized in a supervised manner with respect to a training dataset of input-output pairs.


% %%%%%%%%%%%%%%%%%%%%%%%%%%%%%%%%%%%%%%%%%%%%%%%%%

% % \subsection{Kalman Filter Formulation for the Non-linear Doppler Radar Problem}
% % \label{sec:KF_model_for_radar}

% % Tracking targets from measurements of a Doppler radar is one of the main applications studied in this work.
% % The basic setup of the problem is defined in Section~\ref{sec:setup}.
% % The KF model corresponding to this setup, in terms of Eq.~\ref{eq:KF_model}, is as follows:
% % \begin{equation}
% % \label{eq:KF_for_doppler_radar}
% %     F=\begin{pmatrix} 1 &&& 1 && \\ & 1 &&& 1 & \\ && 1 &&& 1 \\&&& 1 &&\\&&&& 1 &\\&&&&& 1 \end{pmatrix} \qquad H=H(X)=\begin{pmatrix} 1 \\ & 1 \\ && 1 \\ &&& x_x/r & x_y/r & x_z/r \end{pmatrix}
% % \end{equation}
% % where $X=x_{full}$ (in the notation of Section~\ref{sec:setup}) and $r=\sqrt{x_x^2+x_y^2+x_z^2}$. That is, the motion model is the standard constant-velocity model, and the observation model corresponds to direct observation of the location coordinates and a measurement of the radial component of velocity.
% % Note that if observations are received in spherical coordinates, they need to be transformed into Cartesian coordinates before being processed in order to fit the model.

% % Both models ($F,H$) do not depend on the time directly. However, in contrast to the formulation of Eq.~\ref{eq:KF_model}, $H=H(X)$ does depend on the unknown state $X$, and thus $H(X)$ is unknown in inference time. %, and thus the observation model $H(X)\cdot X$ is not linear in $X$.
% % % Furthermore, since the true value of $X$ is unknown to the KF in runtime, $H(X)$ is also unknown.
% % That is, the observation model $h(X)=H(X)\cdot X$ is not linear anymore.
% % The variants of the KF in Section~\ref{sec:OKF} handle this non-linearity as follows:
% % \begin{enumerate}
% %     \item {\bf EKF} is inherently designed to handle such a non-linear model using the approximation $h(X) \approx \tilde{H}\cdot X$, where $\tilde{H}=\nabla_Xh(\hat{X})$ and $\hat{X}$ is the recent estimate of $X$.
% %     \item {\bf KF}: for the standard KF, we use the common trick of approximating $H(X)$ with $\tilde{H}=H(z)$, where $z$ is the recent observation. That is, we replace the unknown location $(x_x,x_y,x_z)$ in Eq.~\ref{eq:KF_for_doppler_radar} with the location coordinates of the observation $(z_x,z_y,z_z)$, resulting in:
% %     $$ \tilde{H}(z) = \begin{pmatrix} 1 \\ & 1 \\ && 1 \\ &&& z_x/\tilde{r} & z_y/\tilde{r} & z_z/\tilde{r} \end{pmatrix} $$
% %     where $\tilde{r}=\sqrt{z_x^2+z_y^2+z_z^2}$. We also implemented other approximations (e.g., $\hat{X}$ instead of $z$), but they did not show added value for the KF baseline in our experiments.
% % \end{enumerate}

% % The KF parameters $Q$ and $R$ were tuned by either Method~\ref{method:KF} (noise-estimation) or Method~\ref{method:OKF} (filtering-errors optimization).
% % Note that both methods are easily applicable to the non-linear setting:
% % \begin{enumerate}
% %     \item Method~\ref{method:KF}: in Eq.~\ref{eq:noise_estimation}, we simply replace $H_t$ with the actual observation model $H(X)$ (note that $X$ \textit{is} available in the training data in our settings).
% %     \item Method~\ref{method:OKF}: as before, we repeatedly run the KF and calculate the gradients of its loss. We simply use the KF (or EKF) implementation explained above.
% % \end{enumerate}


% %%%%%%%%%%%%%%%%%%%%%%%%%%%%%%%%%%%%%%%%%%%%%%%%%
% %%%%%%%%%%%%%%%%%%%%%%%%%%%%%%%%%%%%%%%%%%%%%%%%%

% \section{Generalization Tests: Training and Testing on Different Benchmarks}
% \label{sec:generalization}

% In the case-study of Section~\ref{sec:OKF}, we demonstrate the robustness of an Optimized KF (OKF) over a variety of benchmarks representing different tracking scenarios -- where in every benchmark, OKF (Method~\ref{method:OKF}) obtained lower estimation errors than a standard KF (Method~\ref{method:KF}), {\bf over an out-of-sample test data}.
% This demonstrates that OKF did not overfit the training data, but still relies on representativeness of the training data, i.e., on the assumption that the training data and the test data are taken from the same distribution.

% A stronger generalization ability is demonstrated in Section~\ref{sec:NKF}, where OKF beats both KF and NKF not only on out-of-sample test data with the same settings, but also {\bf on a test data with different settings}. Specifically, we consider changes of factors 0.5 and 2 in the scale of the targets acceleration. This essentially changes the motion of the targets, including turns sharpness, speed changes and typical scale of speed. In terms of the linear motion model of KF, the acceleration corresponds to the motion noise $Q$, hence we essentially changed the noise after it had been learned, which poses a significant generalization challenge.
% Thus, the results of Section~\ref{sec:NKF} provide a significant evidence for the robustness of OKF to certain distributional shifts.

% \begin{figure}[!h]
% \centering
% \begin{subfigure}{\textwidth}
%     \includegraphics[width=\linewidth]{figures/cross_scenarios_detailed.png}
%     \caption{\small $MSE\_ratio = MSE(KF) / MSE(OKF)$ for every KF-baseline (KF,KFp,EKF,EKFp defiend in Section~\ref{sec:OKF}), and for every pair of train-scenario and test-scenario. The colormap is logarithmic ($\sim log(MSE\_ratio)$), where red values represent advantage to OKF ($MSE\_ratio>1$).}
%     \label{fig:cross_scenarios_detailed}
% \end{subfigure}
% \begin{subfigure}{.5\textwidth}
%     \includegraphics[width=\linewidth]{figures/cross_scenarios.png}
%     \caption{\small For every train-scenario, $MSE\_ratio$ is averaged over all the test-scenarios and is shown in a logarithmic scale. Positive values indicate advantage to OKF.}
%     \label{fig:cross_scenarios_summary}
% \end{subfigure}
% \caption{\small Generalization tests: optimization vs. noise estimation under distributional shifts.}
% \label{fig:cross_scenarios}
% \end{figure}

% In this section we present a yet stronger evidence for the robustness of OKF -- not over a parametric distributional shift, but {\bf over entirely different benchmarks}. Specifically, we consider the 5 benchmarks (or scenarios) of Section~\ref{sec:OKF}. For every pair (train-scenario, test-scenario), we train both KF and OKF on data of the train-scenario, then test them on data of the test-scenario.
% For every such pair of scenarios, we measure the generalization advantage of OKF over KF through $MSE\_ratio = MSE(KF) / MSE(OKF)$ (where $MSE\_ratio>1$ indicates positive advantage). To measure the total generalization advantage of a model trained on a certain scenario, we calculate the geometric mean of $MSE\_ratio$ over all the test-scenarios (or equivalently, the standard mean over the logs of the ratios). Note that the logarithmic scale is indeed more natural for a symmetric view of the ratio of the two MSE scores.

% This test is quite noisy, since a model optimized for a certain scenario may legitimately be inferior in other scenarios. Yet, considering all the results together in Figure~\ref{fig:cross_scenarios}, it is evident that optimization of KF yields more robust models in most cases, and even when it \textit{is} inferior to noise-estimation, it does not lose by a large margin.


% %%%%%%%%%%%%%%%%%%%%%%%%%%%%%%%%%%%%%%%%%%%%%%%%%
% %%%%%%%%%%%%%%%%%%%%%%%%%%%%%%%%%%%%%%%%%%%%%%%%%

% \section{Sensitivity of KF Optimization to Train Dataset Size}
% \label{sec:train_size}

% Each benchmark in the case-study of Section~\ref{sec:OKF} has 1500 targets in its train data.
% Training from these datasets demonstrated significant advantage to optimization of KF over noise-estimation.
% However, one may argue that on smaller datasets, optimization may struggle harder than noise-estimation, e.g., due to numeric instability with little data. Furthermore, the standard optimization procedure "wastes" a portion of the train data as a validation set, which does not contribute directly to the training, and thus may increase the sensitivity to the amount of data.

% To test the sensitivity of KF optimization to the amount of data, we repeated some of the tests of Section~\ref{sec:OKF} using smaller subsets of the train datasets -- beginning from as few as 20 targets per dataset.
% Figure~\ref{fig:train_size} demonstrates that the advantage of OKF over KF holds consistently over the various sizes of the train datasets, although it indeed increases with the amount of data.
% In fact, in the Free Motion benchmark, the state-estimation errors of the standard KF monotonously \textit{increase} with the amount of data.

% \begin{figure}[!h]
% \centering
%     \includegraphics[width=0.9\linewidth]{figures/train_size.png}
% \caption{\small The advantage of OKF over KF remains positive -- although sometimes smaller -- even when the train data reduces to as few as 20 targets. The shadowed areas correspond to 95\% confidence-intervals.}
% \label{fig:train_size}
% \end{figure}


% %%%%%%%%%%%%%%%%%%%%%%%%%%%%%%%%%%%%%%%%%%%%%%%%%
% %%%%%%%%%%%%%%%%%%%%%%%%%%%%%%%%%%%%%%%%%%%%%%%%%

% % \section{Optimized Kalman Filter for Video Tracking}
% % \label{sec:MOT20}

% % Radar tracking is an interesting domain with unique properties such as non-linear observation model and radial observation noise.
% % In this domain, Section~\ref{sec:OKF} demonstrates the sub-optimality of KF with estimated noise parameters, compared to a KF with optimized parameters.
% % In this section, we compare the two in the popular and arguably-simpler domain of video tracking, using the MOT20 dataset~\citep{MOT20} (available under \textit{Creative Commons Attribution-NonCommercial-ShareAlike 3.0} License).

% % MOT20 includes several videos with multiple targets (mostly pedestrians) to track.
% % The dataset also includes the ground-truth location and size of the targets in every frame of the videos.
% % We consider these ground-truth states as direct observations, i.e., we assume to have a detector with zero observation error (which in particular makes the observation model linear, in contrast to the radar tracking problem).

% % More specifically, we characterize a target using the state $X=(x,y,w,h,vx,vy)\in \mathbb{R}^6$ (two-dimensional location, size and velocity), and an observation as $Z=(x,y,w,h)$. Note that $x,y,w,h$ are provided in the dataset and we derive $vx,vy$ from $x,y$. The observation model $H$ is known as described above, and for the motion model $F$ we assume constant velocity and constant target size, leading to:
% % $$ H=\begin{pmatrix} 1,0,0,0,0,0 \\ 0,1,0,0,0,0 \\ 0,0,1,0,0,0 \\ 0,0,0,1,0,0 \end{pmatrix}, F=\begin{pmatrix} 1,0,0,0,1,0 \\ 0,1,0,0,0,1 \\ 0,0,1,0,0,0 \\ 0,0,0,1,0,0 \\ 0,0,0,0,1,0 \\ 0,0,0,0,0,1 \end{pmatrix}$$

% % $Q$ and $R$ are estimated or optimized with relation to the train data, as described in Section~\ref{sec:OKF}. For the train data we use MOT20-01,MOT20-02,MOT20-03, and for the test data MOT20-05. In particular, our test data comes from an entirely different video than the train data, hence the testing is less prone to overfit.
% % The goal function for the optimization is the MSE (mean square error) of the location $x,y$ after the prediction step (note that in absence of observation noise, the error of the update step is simply zero).

% % As shown in Figure~\ref{fig:MOT20_res}, the optimized model (OKF) reduces the prediction errors (MSE) by 18\% in comparison to a KF with standard noise estimation.
% % % provides significantly better predictions than KF with standard noise estimation, and reduces the MSE by 18\%.
% % The significance level of the results is also indicated by the huge z-value $z=125$, corresponding to the errors difference (calculated as $z=mean(\Delta err)/std(\Delta err)\cdot\sqrt{N_{samples}}$).
% % The results indicate that the sub-optimality of noise estimation -- as well as the benefits of parameters optimization -- are a cross-domain phenomenon and are not limited to radar tracking or to non-linear observation models.

% % % \begin{figure}[!h]
% % % \centering
% % % \begin{subfigure}{.39\textwidth}
% % %     \includegraphics[width=\linewidth]{figures/MOT20/MOT20_SE.jpg}
% % %     \label{fig:MOT20_res}
% % % \end{subfigure}
% % % \begin{subfigure}{.6\textwidth}
% % %     \includegraphics[width=\linewidth]{figures/MOT20/MOT20_sample.jpg}
% % %     \label{fig:MOT20_sample}
% % % \end{subfigure}
% % % \caption{\small (a) Prediction errors of KF and OKF on 1208 targets of the test data of MOT20. OKF is clearly more accurate, as also indicated by the huge z-value corresponding to the errors difference (calculated as $z=mean(\Delta err)/std(\Delta err)\cdot\sqrt{N}$). (b) A sample of 2 targets in the first frame of MOT20 test data. The true trajectories are shown along with the predictions of KF and OKF (each prediction is done one time-step in advance).}
% % % \end{figure}

% % % \begin{figure}[!h]
% % % \centering
% % % \includegraphics[width=.5\linewidth]{figures/MOT20/MOT20_SE.jpg}
% % % \caption{\small Summary of the prediction errors of KF and OKF on 1208 targets of the test data of MOT20. The errors of OKF are clearly smaller than those of KF, as also indicated by the huge z-value corresponding to the errors difference (calculated as $z=mean(\Delta err)/std(\Delta err)\cdot\sqrt{N}$).}
% % % \label{fig:MOT20_res}
% % % \end{figure}

% % \begin{figure}[!h]
% % \centering
% % \includegraphics[width=.7\linewidth]{figures/MOT20/MOT20_sample.jpg}
% % \caption{\small A sample of 2 targets in the first frame of the test video in MOT20. The true trajectories of the targets are shown along with the predictions of KF and OKF (each prediction is done one time-step in advance).}
% % \label{fig:MOT20_sample}
% % \end{figure}


% % %%%%%%%%%%%%%%%%%%%%%%%%%%%%%%%%%%%%%%%%%%%%%%%%%
% % %%%%%%%%%%%%%%%%%%%%%%%%%%%%%%%%%%%%%%%%%%%%%%%%%

% % \section{Optimized Kalman Filter for Lidar-based State Estimation in Self Driving}
% % \label{sec:lidar}

% % Another domain in which we test the Optimized Kalman Filter (OKF) of Section~\ref{sec:OKF} is state-estimation in self-driving based on lidar measurements with respect to known landmarks~\citep{lidar_from_beacons}.
% % For simplicity, we focus on location estimation and on a single landmark (as the matching problem from multiple landmarks is out of the scope of this work).

% % We formulate the problem as follows: the target state is $X=(x,y,vx,vy)\in \mathbb{R}^4$ (two-dimensional location and velocity), and an observation is $Z=(x,y)$. The dynamics are simulated as follows: each target trajectory consists of several intervals, in each one the target has certain (positive or negative) acceleration and certain lateral acceleration ("turn magnitude"), both drawn randomly at the beginning of the interval. The observation noise is drawn i.i.d in polar coordinates.
% % We simulated a corresponding dataset of 2000 targets as demonstrated in Figure~\ref{fig:lidar_trajectories}, and split them to train set (1400 targets) and test set (600 targets).

% % From the KF point-of-view, the dynamics and observations are modeled by:
% % $$ H=\begin{pmatrix} 1,0,0,0 \\ 0,1,0,0 \end{pmatrix}, F=\begin{pmatrix} 1,0,1,0 \\ 0,1,0,1 \\ 0,0,1,0 \\ 0,0,0,1 \end{pmatrix}$$
% % Note that the lidar problem is inherently different from the radar problem (Section~\ref{sec:OKF}) since the observation model is linear (due to the absence of the Doppler signal); and is different from video tracking (as formulated in Appendix~\ref{sec:MOT20}) since the observations are not assumed to be noiseless.
% % On the other hand, similarly to the case of the radar, the Cartesian representation of the observations prevents their noise from being i.i.d, since the observation noise is only i.i.d in polar coordinates (see Appendix~\ref{sec:polar_coordinates}).

% % We trained the OKF of Section~\ref{sec:OKF} with respect to the MSE of the estimated target location, as described in Appendix~\ref{sec:training}; and trained a standard KF by estimating the noise as in Eq.~\ref{eq:noise_estimation}.
% % Then we tested both models on the test data.
% % The optimization significantly reduced the errors by 14.9\%, as shown in Figure~\ref{fig:lidar_MSE}.
% % This joins the promising results from the two other domains (radar tracking and video tracking), and demonstrates the generality of our method.

% % \begin{figure}[!h]
% % \centering
% % \begin{subfigure}{.33\textwidth}
% %     \includegraphics[width=\linewidth]{figures/lidar/lidar_trajectories.png}
% %     \caption{}
% %     \label{fig:lidar_trajectories}
% % \end{subfigure}
% % \begin{subfigure}{.32\textwidth}
% %     \includegraphics[width=\linewidth]{figures/lidar/lidar_MSE.png}
% %     \caption{}
% %     \label{fig:lidar_MSE}
% % \end{subfigure}
% % \begin{subfigure}{.3\textwidth}
% %     \includegraphics[width=\linewidth]{figures/lidar/lidar_sample.png}
% %     \caption{}
% %     \label{fig:lidar_sample}
% % \end{subfigure}
% % \caption{\small (a) A sample of 6 targets trajectories from the simulated self-driving data. (b) Prediction errors of KF and OKF on 600 targets of the test data. OKF is clearly more accurate, as also indicated by the huge z-value corresponding to the errors difference (calculated as $z=mean(\Delta err)/std(\Delta err)\cdot\sqrt{N}$). (c) the tracking of KF and OKF on a sample target trajectory, focused on the time interval $14<t<32$ for visual clarity.}
% % \end{figure}


% %%%%%%%%%%%%%%%%%%%%%%%%%%%%%%%%%%%%%%%%%%%%%%%%%
% %%%%%%%%%%%%%%%%%%%%%%%%%%%%%%%%%%%%%%%%%%%%%%%%%

% \section{Neural Kalman Filter: Extended Experiments}
% \label{sec:NKF_extended}

% Section~\ref{sec:NKF} demonstrates that even if a neural-network (NN) based model provides more accurate predictions than a standard KF -- its advantage may be entirely vanished when compared to an optimized KF instead.
% It is shown for the specific NKF model in a free-motion benchmark in the Doppler radar problem.
% This is sufficient to demonstrate the error in the common methodology that compares optimized NN-based models to non-optimized variants of KF.

% To show that these results are not exclusive to the experiments of Section~\ref{sec:NKF}, we present extended experiments in this section.
% Specifically, we consider 2 different benchmarks -- the free-motion benchmark of Section~\ref{sec:NKF} and Const\_a benchmark of Section~\ref{sec:OKF} (in which the targets may have acceleration but not turns). We also consider 3 different neural models:
% \begin{itemize}
%     \item Predicted-acceleration KF (aKF): a variant of NKF without dynamic prediction of the covariance matrices $Q$ and $R$ in every step.
%     \item Neural KF (NKF): the model used in Section~\ref{sec:NKF} and shown in Figure~\ref{fig:NKF_diagram}.
%     \item Neural KF with H-prediction (NKFH): a variant of NKF that also predicts the observation model $H$ dynamically in every step.
% \end{itemize}

% For each benchmark and each model, we trained the model on train data with a certain range of targets acceleration (note that acceleration affects both speed changes and turns sharpness), and tested it on targets with three different acceleration ranges -- the original one, a smaller one and a larger one. That is, some of the test datasets correspond to distributional shifts.
% For each model we train two variants -- one with Cartesian representation of the observation noise $R$, and one with spherical representation (as in the baselines of Section~\ref{sec:OKF}) -- and we select the best among the two variants using the MSE scores on the validation data (which is a portion of the data assigned for training).

% We measure the results using (1) the Mean Square Error (MSE) of the estimated location after each update step; and (2) the Negative-Log-Likelihood (NLL) of the true system-state with relation to the estimated state-distribution, after the prediction step. Note that NLL is important for matching observations to targets in the multi-target tracking problem (which is out of the scope of this work).

% \begin{figure}[!h]
% \centering
% \begin{subfigure}{\textwidth}
%     \includegraphics[width=\linewidth]{figures/NKF_Free_paired_res.png}
%     \caption{\small Free-motion benchmark}
%     \label{fig:NKF_extended_free}
% \end{subfigure}
% \begin{subfigure}{\textwidth}
%     \includegraphics[width=\linewidth]{figures/NKF_Consta_paired_res.png}
%     \caption{\small Const\_a benchmark (no turns)}
%     \label{fig:NKF_extended_consta}
% \end{subfigure}
% \caption{\small The \textit{relative} MSE and NLL results of various models in comparison to the standard KF model. The textual labels specify the \textit{absolute} MSE and NLL. Note that certain bars of NLL are of entirely different scale and thus are cropped in the figure (their values can be seen in the labels).
% In each benchmark, the models were trained with relation to MSE loss, on train data of the middle acceleration-range: the two other acceleration ranges in each benchmark correspond to generalization over distributional shifts.}
% \label{fig:NKF_extended}
% \end{figure}

% Figure~\ref{fig:NKF_extended_free} shows that in the free-motion benchmark, all the 3 neural models improve the MSE in comparison to a standard KF, but lose to an optimized one (OKF).
% Furthermore, while OKF has the best NLL scores, the more complicated models NKF and NKFH increase the NLL in orders of magnitude. This issue may be handled by explicitly optimize the NLL in addition to the MSE, but such multi-loss optimization is out of the scope of this work.
% Note that the instability of NKFH is expressed in poor generalization to lower accelerations in addition to the extremely high NLL score.

% Figure~\ref{fig:NKF_extended_free} shows that in Const\_a benchmark, all the 3 neural models improve the MSE in comparison to a standard KF, but only NKFH improves in comparison to OKF as well.
% Note that while NKFH does better in this case than in the free-motion benchmark, it still suffers from very high NLL.

% In summary, by comparing the optimized neural models to the standard KF model, all the 3 models would be found superior to the KF in both benchmarks in terms of MSE. However, when shifting the baseline to an \textit{optimized} KF, we find that the neural aKF and NKF are in fact inferior to OKF, and that the comparison between NKFH and OKF depends on the selected benchmark and metric.

% Of course, our results do not imply that neural-networks in general cannot be superior to a KF: only that when comparing the two, one must optimize the KF similarly to the neural model to avoid misleading experimental results. As discussed in Section~\ref{sec:related_work}, the wrong methodology of using a non-optimized KF baseline is very common in the literature.


% %%%%%%%%%%%%%%%%%%%%%%%%%%%%%%%%%%%%%%%%%%%%%%%%%
% %%%%%%%%%%%%%%%%%%%%%%%%%%%%%%%%%%%%%%%%%%%%%%%%%

% \section{On the Guarantees of Gradient-based Optimization}
% \label{sec:GD_limitations}

% Method~\ref{method:OKF} can rely on any gradient-based optimization algorithm, such as SGD or Adam~\citep{adam} (the latter is used in this work).
% Such optimization algorithms have achieved remarkable results in a variety of optimization problems in the recent years. This includes impressive results in non-convex problems where local-minima exist~\citep{adam_revisited}, as well as generalization to unseen data~\citep{GD_generalization}.

% Compared to the problems where algorithms like Adam are often applied (e.g., language models with more than 100M parameters~\citep{bert}), typical filtering problems such as the ones experimented in this work are arguably small and simple to optimize.
% Thus, the robust results of Method~\ref{method:OKF} -- namely, the consistent advantage over Method~\ref{method:KF} in \textit{all} the experiments in this work -- should not come as a surprise.

% Having said that, the \textit{theoretical} guarantees of the gradient-based algorithms are limited for non-convex problems.
% Note that the dependence of our loss function (filtering errors) on the model parameters (after the Cholesky parameterization) is indeed not convex.
% In such settings, convergence to a local optimum of the loss \textit{is} in fact guaranteed: Adam, for example, is guaranteed to converge given a twice-differentiable loss function~\citep{adam_convergence}.
% Stronger convergence guarantees exist for the SGD algorithm under certain conditions~\citep{SGD_convergence}, yet in general, gradient-based optimization algorithms do not necessarily converge to the global optimum of the loss.
% Furthermore, the global optimum is not necessarily unique.

% Note that in all the problems experimented in this work, the standard Method~\ref{method:KF} (noise-estimation) has no optimality guarantee either, as the KF assumptions do not hold.
% Indeed, the experiments demonstrate its sub-optimality, and Appendices~\ref{sec:toy_analysis},\ref{sec:theory_noniid} prove it theoretically for a sample of problems.


% %%%%%%%%%%%%%%%%%%%%%%%%%%%%%%%%%%%%%%%%%%%%%%%%%
% %%%%%%%%%%%%%%%%%%%%%%%%%%%%%%%%%%%%%%%%%%%%%%%%%

% \section{Detailed Results}
% \label{sec:detailed_results}

% Figures~\ref{fig:res_OKF_detailed}-\ref{fig:benchmarks_EDA} below provide additional details about the experiments discussed in Sections~\ref{sec:OKF},\ref{sec:NKF}.

% % \begin{figure}[!h]
% % % \vspace{-10pt}
% % \centering
% % % \begin{subfigure}{.4\textwidth}
% % %   \centering
% %   \includegraphics[width=.35\linewidth]{figures/NKF_NLL.png}
% % %   \caption{}
% % % \end{subfigure}
% % % \begin{subfigure}{.3\textwidth}
% % %   \centering
% % %   \includegraphics[width=1.\linewidth]{figures/oracle_NLL.jpg}
% % %   \caption{}
% % % \end{subfigure}
% % \caption{\footnotesize Negative-log-likelihood errors of different tracking models, over targets with different ranges of acceleration. This is analog to Figure~\ref{fig:res_NKF_MSE}, but measures NLL rather than MSE.}
% % % \caption{\footnotesize Negative-log-likelihood errors of different tracking models, over (a) targets with different ranges of acceleration, and (b) different benchmarks. These are analog to Figures~\ref{fig:res_NKF_MSE} and \ref{fig:res_oracle_MSE}, but measure NLL rather than MSE.}
% % \label{fig:res_NKF_NLL}
% % \end{figure}

% \begin{figure}[h]%[b]
% % \vspace{-10pt}
% \centering
% \begin{subfigure}{.8\textwidth}
%   \centering
%   \includegraphics[width=1.\linewidth]{figures/res_all_KF.png}
%   \caption{}
%   \label{fig:res_all_KF}
% \end{subfigure} \\
% \begin{subfigure}{.45\textwidth}
%   \centering
%   \includegraphics[width=1.\linewidth]{figures/res_relative.png}
%   \caption{}
%   \label{fig:res_relative}
% \end{subfigure}
% \caption{\footnotesize (a) Errors of different tracking models over different benchmarks. This is a different visualization of the results of Table~\ref{tab:res_OKF}. The error-bars correspond to confidence intervals of 95\%. Note that each of the optimized models (the last four) consistently yields lower errors than the corresponding estimated model (among the first four) -- in most cases with high statistical significance. (b) The RMSE ratio between the estimated models and the optimized ones, over all the benchmarks and designs discussed in Section~\ref{sec:OKF}. Note that all the ratios are above 1, i.e., all the models in all the benchmarks had smaller errors when tuned by optimization. The horizontal line represents the average ratio.}
% \label{fig:res_OKF_detailed}
% \end{figure}

% \begin{figure}[!h]
% % \vspace{-10pt}
% \centering
% \begin{subfigure}{.24\textwidth}
%   \centering
%   \includegraphics[width=1.\linewidth]{figures/noise_R_Free_KF.png}
%   \caption{\footnotesize $R$ (estimated)}
%   \label{fig:noise_R_KF}
% \end{subfigure}
% \begin{subfigure}{.24\textwidth}
%   \centering
%   \includegraphics[width=1.\linewidth]{figures/noise_R_Free_OKF.png}
%   \caption{\footnotesize $R$ (optimized)}
%   \label{fig:noise_R_OKF}
% \end{subfigure}
% \begin{subfigure}{.24\textwidth}
%   \centering
%   \includegraphics[width=1.\linewidth]{figures/noise_Q_Free_KF.png}
%   \caption{\footnotesize $Q$ (estimated)}
%   \label{fig:noise_Q_KF}
% \end{subfigure}
% \begin{subfigure}{.24\textwidth}
%   \centering
%   \includegraphics[width=1.\linewidth]{figures/noise_Q_Free_OKF.png}
%   \caption{\footnotesize $Q$ (optimized)}
%   \label{fig:noise_Q_OKF}
% \end{subfigure}
% \caption{\footnotesize The observation noise ($R$) and prediction noise ($Q$) matrices obtained in a (Cartesian) KF by noise estimation and by optimization with relation to $MSE$, based on the dataset of the Free-motion benchmark.}
% \label{fig:noise_params}
% \end{figure}

% \begin{figure}[!h]
% % \vspace{-10pt}
% \centering
% % \begin{subfigure}{.32\textwidth}
% %   \centering
% %   \includegraphics[width=1.\linewidth]{figures/tars_Toy.png}
% % \end{subfigure}
% \begin{subfigure}{.32\textwidth}
%   \centering
%   \includegraphics[width=1.\linewidth]{figures/tars_Close.png}
% \end{subfigure}
% \begin{subfigure}{.32\textwidth}
%   \centering
%   \includegraphics[width=1.\linewidth]{figures/tars_Const_v.png}
% \end{subfigure} %\\
% \begin{subfigure}{.32\textwidth}
%   \centering
%   \includegraphics[width=1.\linewidth]{figures/tars_Const_a.png}
% \end{subfigure}
% % \begin{subfigure}{.32\textwidth}
% %   \centering
% %   \includegraphics[width=1.\linewidth]{figures/tars_Free.png}
% % \end{subfigure}
% \caption{\footnotesize Samples of targets trajectories in the various benchmarks described in Section~\ref{sec:OKF}, projected onto the horizontal plane. This is an extension of Figures~\ref{fig:trajectories_toy},\ref{fig:trajectories_free} for the rest of the benchmarks.}
% \label{fig:all_trajectories}
% \end{figure}

% \begin{figure}[!h]
%   \centering
%   \includegraphics[width=1.\linewidth]{figures/benchmarks_EDA.png}
%     \caption{\footnotesize Descriptive statistics of the various benchmarks of Section~\ref{sec:OKF}: duration of targets trajectories; distance from the radar; targets speed; targets acceleration; motion direction (90 degrees correspond to horizontal motion); and observation errors vs. distance from radar.}
%     \label{fig:benchmarks_EDA}
% \end{figure}


% %%%%%%%%%%%%%%%%%%%%%%%%%%%%%%%%%%%%%%%%%%%%%%%%%
% %%%%%%%%%%%%%%%%%%%%%%%%%%%%%%%%%%%%%%%%%%%%%%%%%

% \bibliographystyle{plainnat}
% % \nocite{*}
% \bibliography{main}


% \end{document}
